# Supplementary material for: Effectiveness of 3VQM in Capturing Depth Inconsistencies
Source: arXiv:1811.08817 ancillary file (2018-11-21)
Supplement: Supplementary file 1 [file Temel2013_IVMSP.pdf]

# **Effectiveness of 3VQM in Capturing Depth Inconsistencies**

Dogancan Temel and Ghassan AlRegib

Multimedia and Sensors Lab (MSL)  
School of Electrical and Computer Engineering  
Georgia Institute of Technology  
June 10, 2013

1. A 3D Video Quality Measure (3VQM)
2. Validation of 3VQM
3. Performance Evaluation of 3VQM

# A 3D Video Quality Measure (3VQM)

Stereoscopic 3D

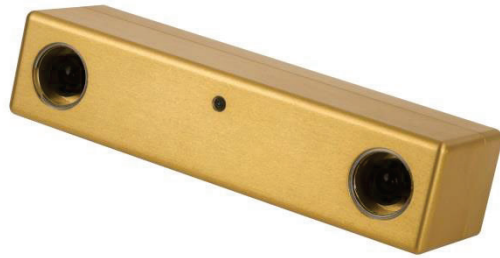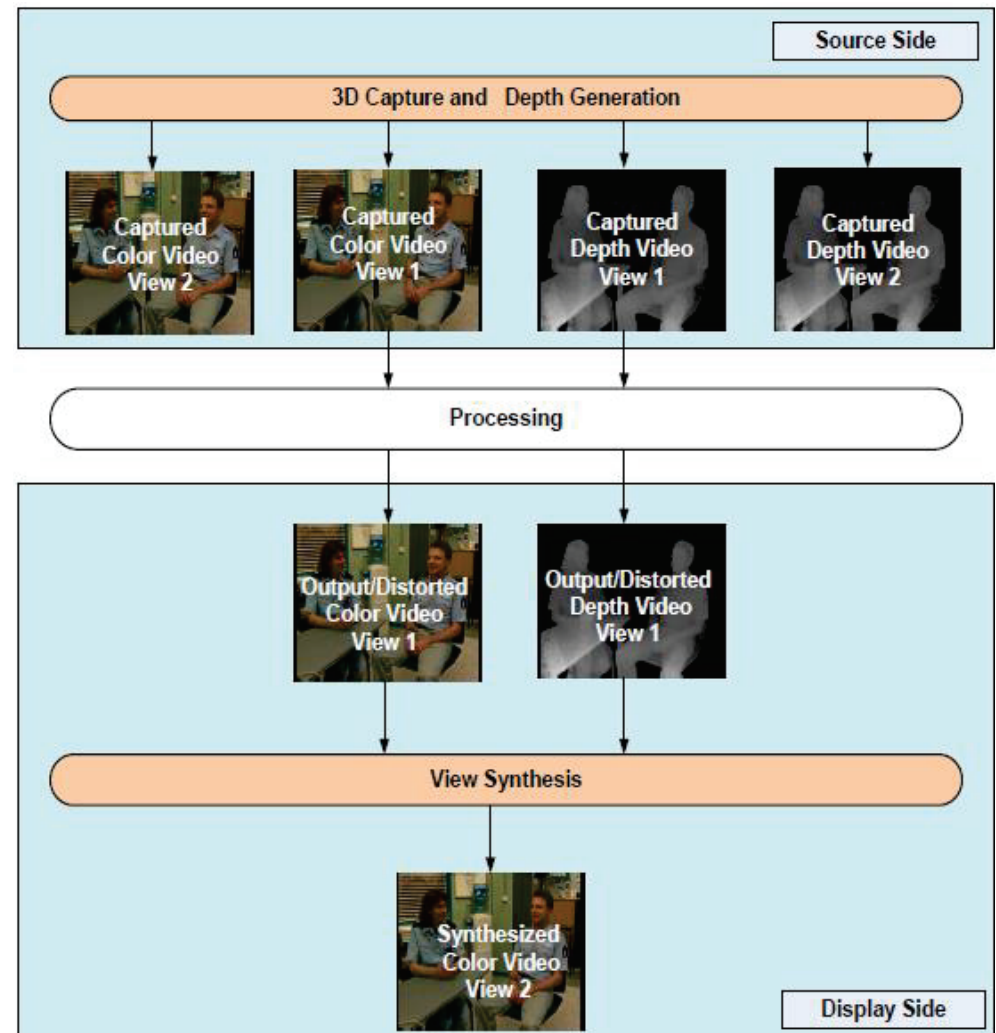

# A 3D Video Quality Measure (3VQM)

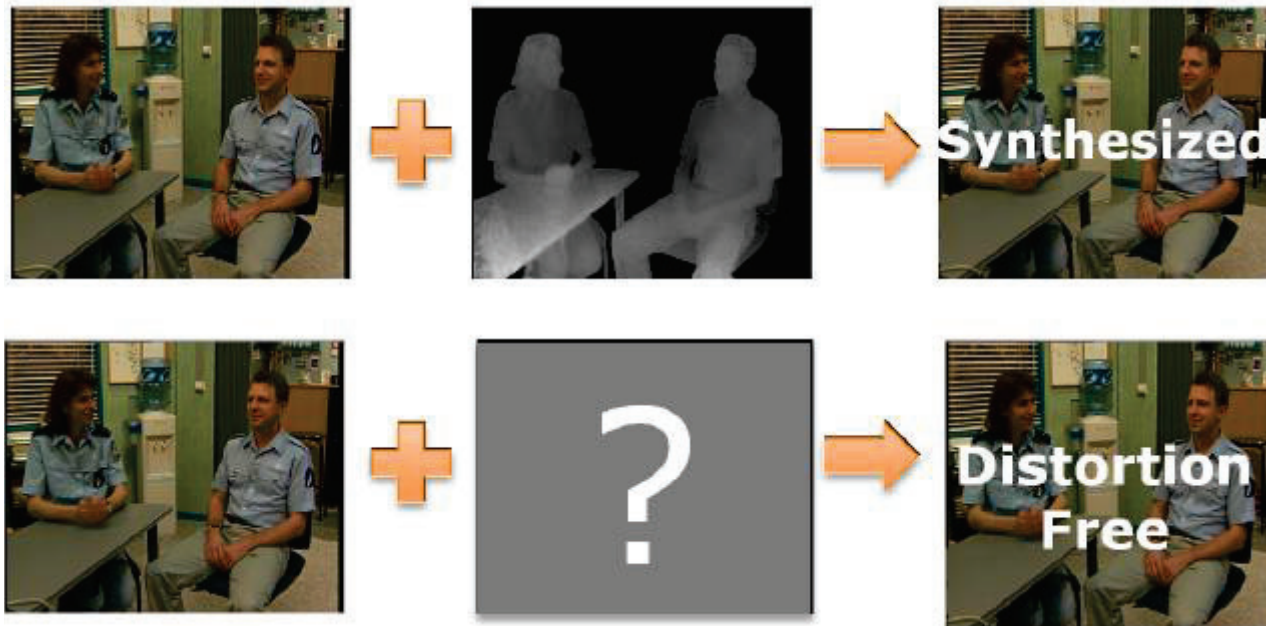

# A 3D Video Quality Measure (3VQM)

## 3D Wrapping

$$X_v = X_r + s \frac{F_v B}{Z} + h, \quad h = -s \frac{F B}{Z_c}$$

$$X_o = X_r + s \frac{F_v B}{Z_{ideal}} + h,$$

$$Z_{ideal} = \frac{s F_v B}{(X_o - X_v) + s \frac{F_v B}{Z}}$$

$$Z_{ideal} \approx \frac{s F_v B}{\alpha(I_o - I_v) + \frac{s F_v B}{Z}}$$

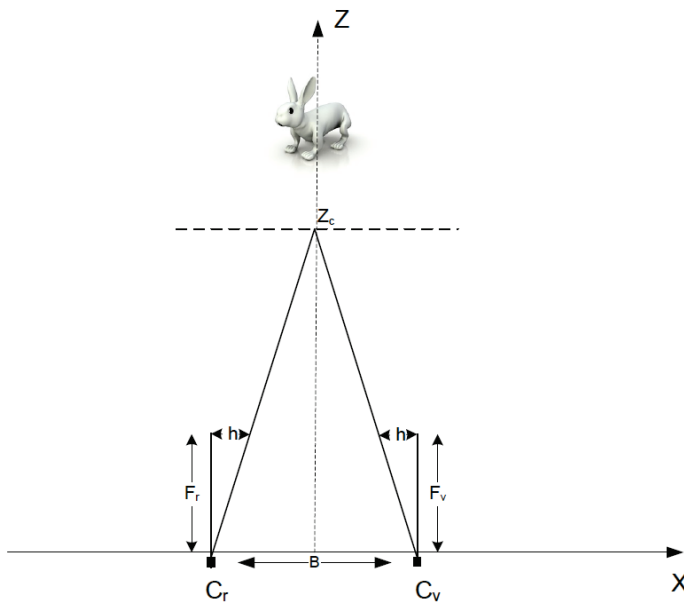

# A 3D Video Quality Measure (3VQM)

$$\Delta Z = |Z_{ideal} - Z|$$

**Spatial Outliers (SO)**  
 $STD(\Delta Z)$

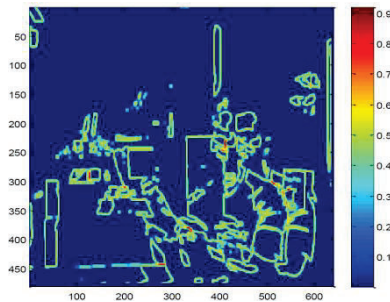

**Temporal Outliers (TO)**  
 $STD(\Delta Z_K - \Delta Z_{K-1})$

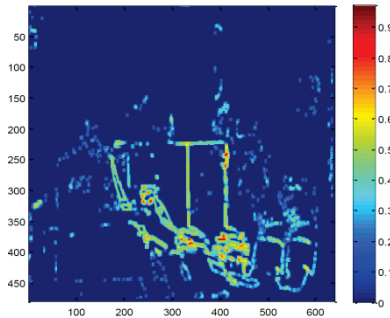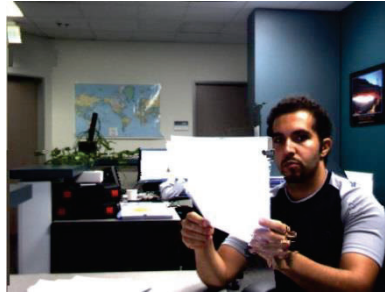

**Temporal Inconsistencies (TI)**  
 $STD(Z_K - Z_{K-1})$

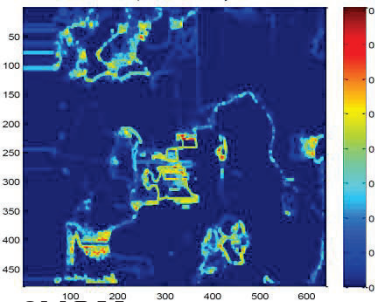

**3VQM**

$$K(1 - SO(SO \cap TO))^a(1 - TI)^b(1 - TO)^c$$

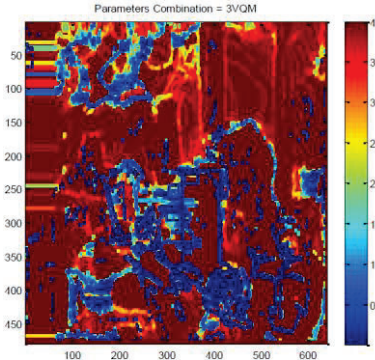

1. A 3D Video Quality Measure (3VQM)
- 2. Validation of 3VQM**
3. Performance Evaluation of 3VQM

# Validation of 3VQM

**RMSE:** Root Mean Squared Error

**CC:** Pearson Linear Correlation Coefficient

**ROCC:** Spearman Rank Order Correlation Coefficient

**MAE:** Mean Absolute Error

**Low RMSE:** Accuracy

**High CC:** Coherency

**High ROCC:** Coherency

**Low MAE:** Accuracy

|                       | RMSE | CC   | ROCC | MAE  |
|-----------------------|------|------|------|------|
| Average PSNR          | 0.95 | 0.73 | 0.72 | 0.82 |
| Weighted Average PSNR | 0.94 | 0.76 | 0.78 | 0.79 |
| Average SSIM          | 0.81 | 0.60 | 0.54 | 0.62 |
| 3VQM                  | 0.62 | 0.89 | 0.79 | 0.52 |



# Validation of 3VQM

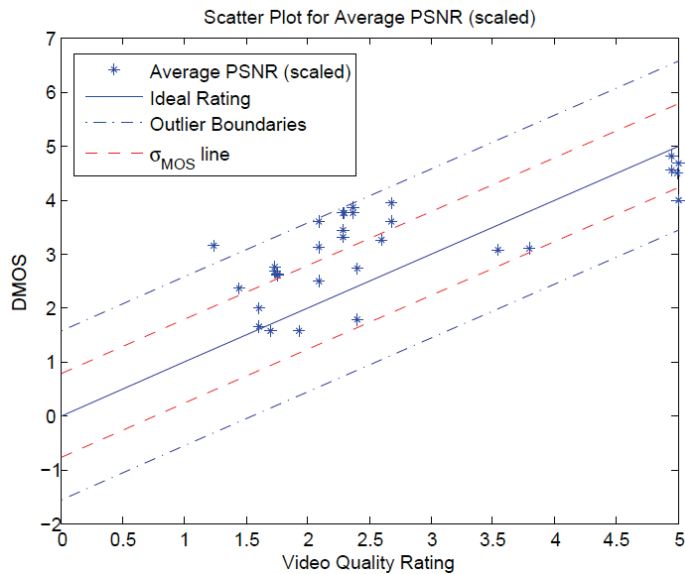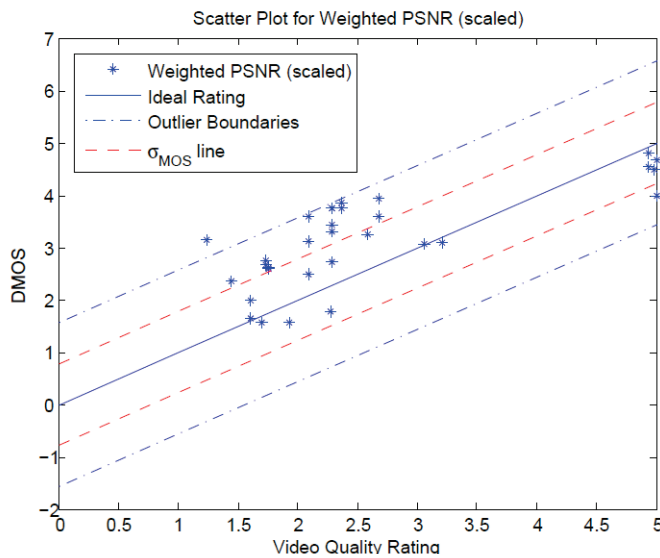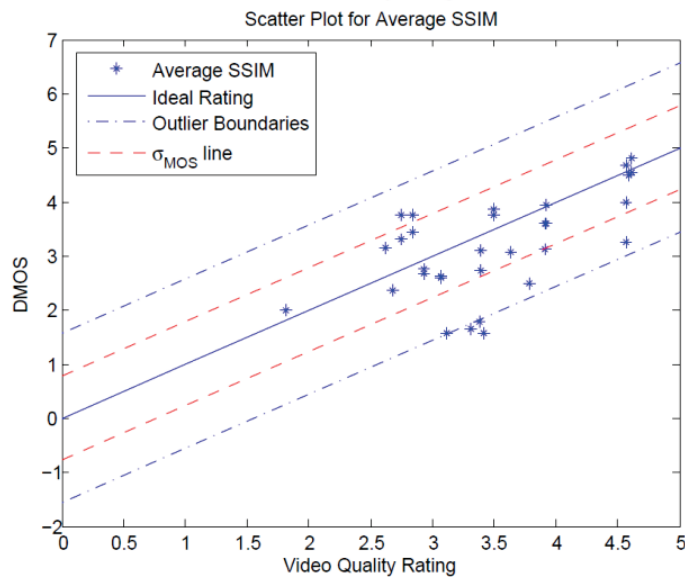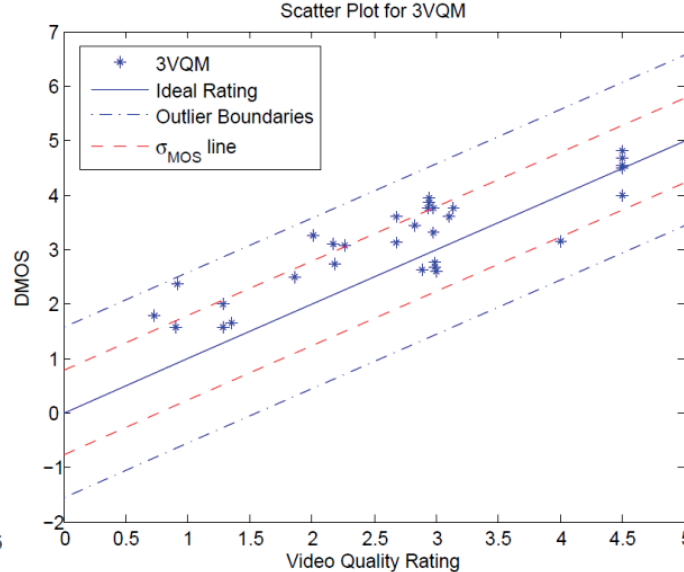

OR: Outlier Ratio    Low OR: Consistency

|                       | OR   |
|-----------------------|------|
| Average PSNR          | 0.19 |
| Weighted Average PSNR | 0.19 |
| Average SSIM          | 0.13 |
| 3 VQM                 | 0.00 |

1. A 3D Video Quality Measure (3VQM)
2. Validation of 3VQM
3. **Performance Evaluation of 3VQM**

# Performance Evaluation of 3VQM

## Blur

Gaussian Blur Kernel

| Kernel Size / Standard deviation | $\sigma_1$ | $\sigma_2$ | $\sigma_3$ |
|----------------------------------|------------|------------|------------|
| 7x7                              | 2          | 5          | 10         |
| 19x19                            | 10         | 20         | 80         |

## Compression

Type: H.264, Coding method: Entropy

| Quantization Parameter (QP) | 28 | 40 | 50 |
|-----------------------------|----|----|----|
|-----------------------------|----|----|----|

## Transmission

Model: Gilbert Elliot

| Packet Loss Rate | 2 % | 5 % | 10 % |
|------------------|-----|-----|------|
|------------------|-----|-----|------|

# Performance Evaluation of 3VQM

## Blur

Depth

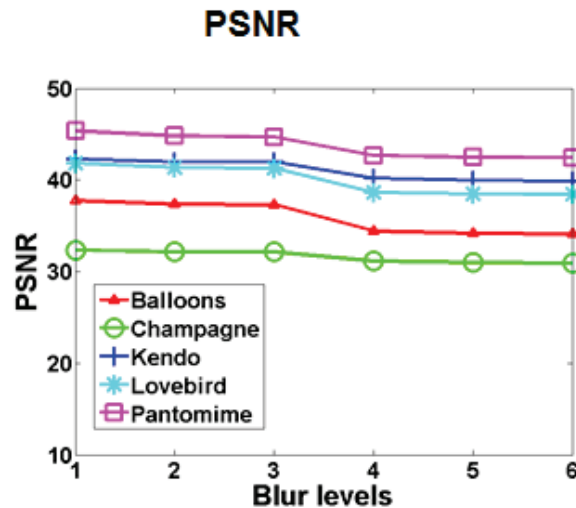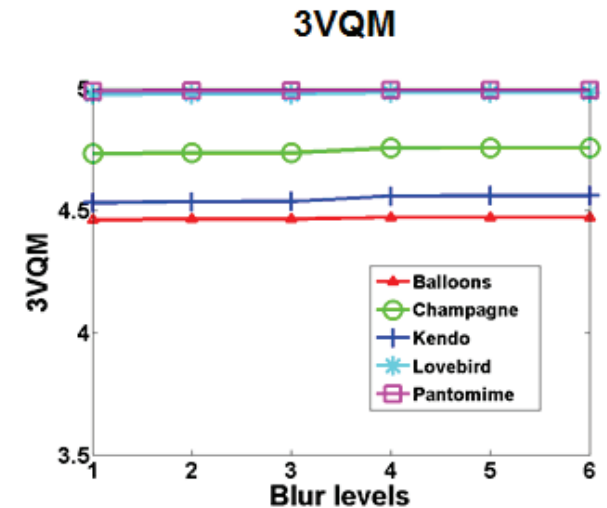

Color

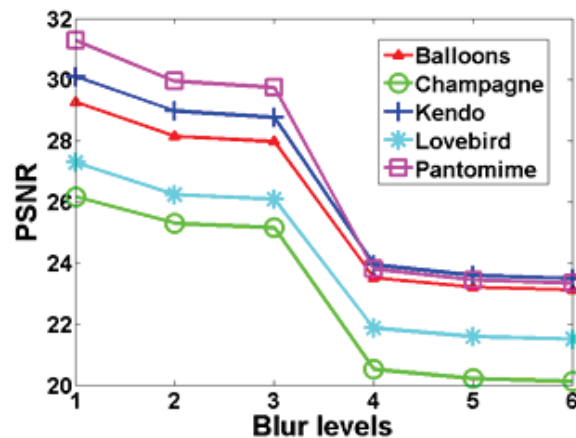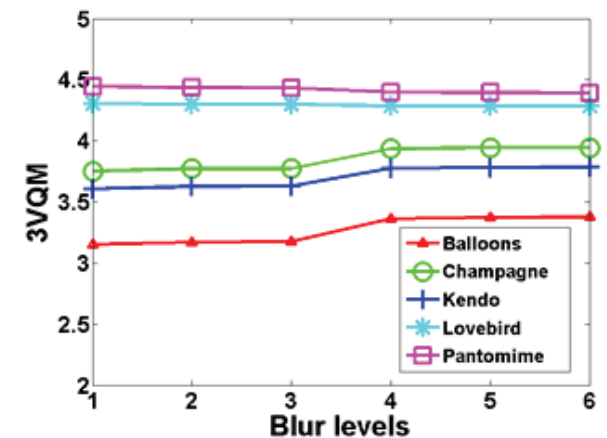

# Performance Evaluation of 3VQM

## Compression

Depth

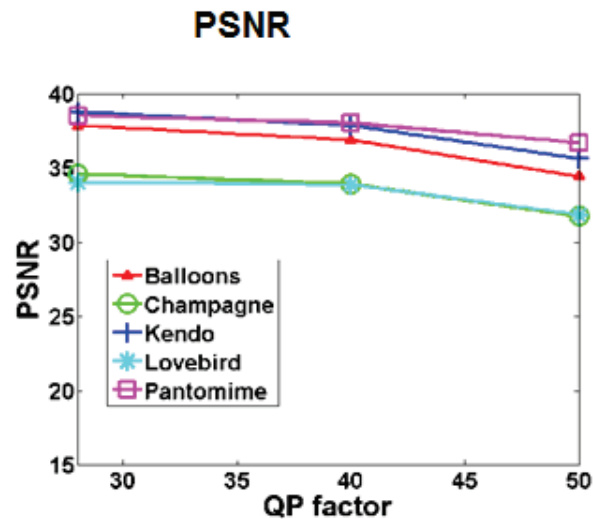

Color

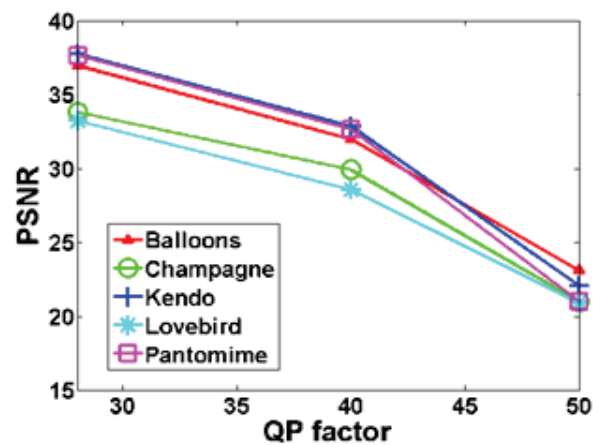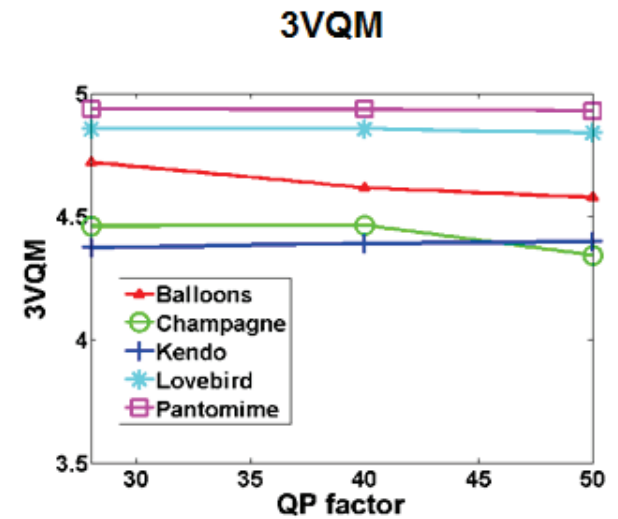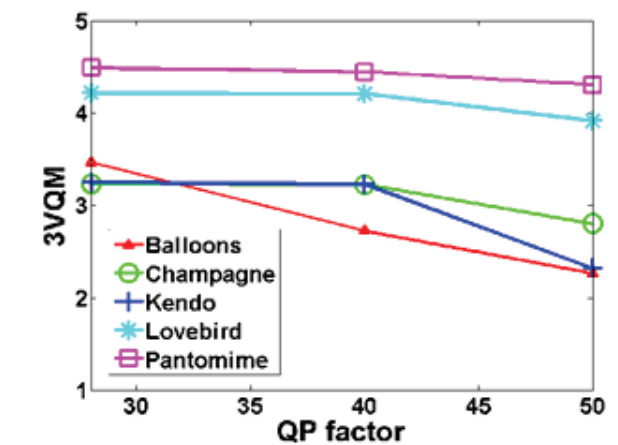

# Performance Evaluation of 3VQM

## Transmission

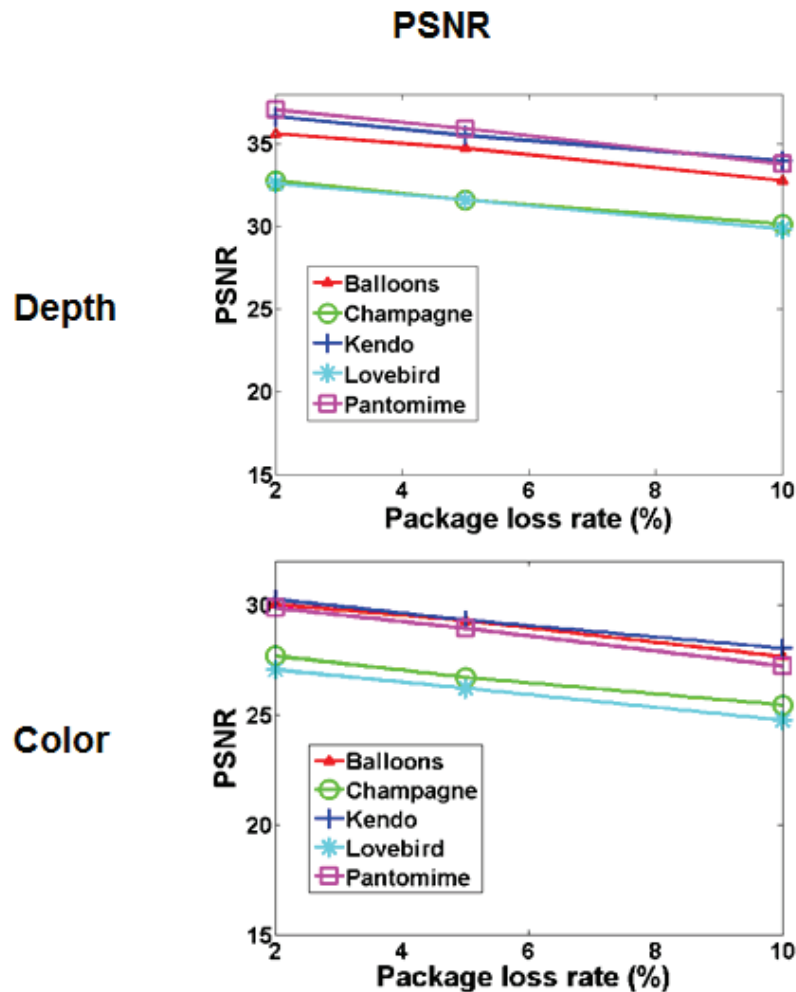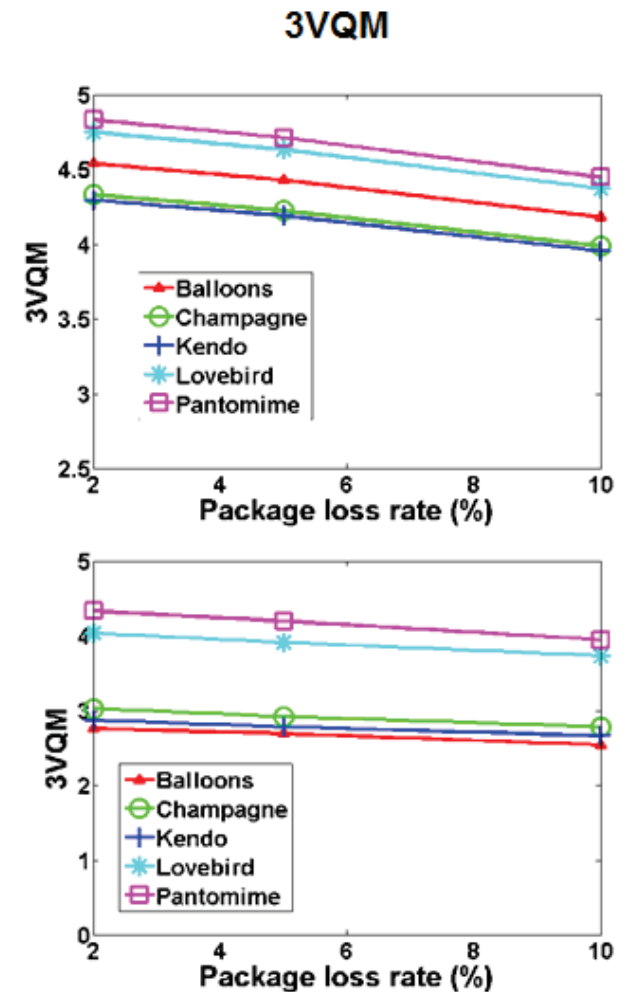

## To summarize

### **3VQM is**

- Accurate
- Coherent
- Consistent

### **3VQM is sensitive to**

- Compression artifacts in color video
- Transmission artifacts

### **3VQM is not sensitive to**

- Blurring artifacts
- Compression artifacts in depth
